# Supplementary material for: Multi-Task Partially Supervised Learning for Super-Resolution and Semantic Segmentation on Earth Observation data
Source: arXiv:2610.06389 source file (2026-10-05)
Supplement: Supplementary file 1 [file A_supp.tex]

\section{Architecture}

    \begin{figure*}[h]
        \centering
        \def\svgwidth{\linewidth}
        \large
        \input{Images/SQ2.pdf_tex}
        \caption{The \textit{hybrid} architecture includes a shared backbone and an extended head sequentially placed after super-resolution, fusing them into the segmentation head. Scattering is performed after the corresponding transition, and gathering after fusion.}
        \label{fig:SQHead_supp}
    \end{figure*}

    We are now detailing the scatter and gather operators in the hybrid architecture which can be seen in Figure~\ref{fig:SQHead_supp}. For the sake of brevity, the RRDB encoder and convolutional blocks are removed.
    The scatter operator comprises mainly downsampling operators which are a convolutional layer with a kernel size of 3 and a stride of 2, followed by a batch normalization layer. On the other hand, the gather operator consists of upsampling  operators which are
    $1\times1$-convolution followed by a batch normalization and a $2\times$-bilinear upsampling.
    In Figure~\ref{fig:SQHead_supp}, the scatter and gather operation are shown above a transition (in {\color[HTML]{0044aa}blue}) and a fusion layer (in {\color[HTML]{ff55dd}{magenta}}), yet they should be implemented in the antecedent of these layers.
    The super-resolved image produced by the super-resolution head is first downsampled by half and embedded using the same downsampling block before going to a scatter layer.
    A scatter layer receives the features from the previous layer in the super-resolution branch, downsamples and adds them to each of the semantic features at each scale before passing to the corresponding {\color[HTML]{0044aa} transition layer}.
    Conversely, a gather layer receives the features before going into the corresponding {\color[HTML]{ff55dd} fusion layer}, upsamples and adds them to the super-resolution branch.
    

\section{Dataset}

The ISPRS 2D semantic labeling contest~\cite{isprs2012} and the proprietary datasets using real and synthetic Pléiades imagery are employed for experimentation.

\textbf{The ISPRS dataset\footnote{[Online] ISPRS, 2D semantic Labeling Context, accessed June 2024. \url{https://www.isprs.org/education/benchmarks/UrbanSemLab/semantic-labeling.aspx}.}} comprises aerial images of two cities, Vaihingen and Potsdam, with typical differences found in remote sensing datasets. As shown in Figure~\ref{fig:ISPRS_visual_SM}, besides the diverse sensor specifications, distinctive geographical characteristics also lead to varied distributions: the small village Vaihingen appears with detached houses and reddish vegetation due to IR-R-G sensors, while the historic city Potsdam has complex buildings and narrow streets.
The Vaihingen images taken with a ground sampling distance (GSD) of 9cm are provided in 33 tiles of resolution around 3K$\times$2K,
whereas the Potsdam images are taken at a GSD of 5cm and provided in 38 tiles of 6K$\times$6K pixels.
The data are split into training and testing splits following the conventional setting and will be released upon acceptance.
The IR-R-G bands are used to match Potsdam images with Vaihingen's.

In our experiments, we study two scenarios: (1) the partial multi-task (PMTL) only and (2) with the blind super-resolution (BSR). Concerning the former specifically, a hypothetical pair setting is adopted, where a natural LR counterpart $L_R$ with representative degradations is available for each training HR image $H_R$.

For both cases, the clean super-resolution (CSR) evaluation strategy proposed in~\cite{Lugmayr2019} is employed for evaluating super-resolution. In particular, the testing data are simulated by degrading clean HR images with hidden kernels and injecting noise of unknown statistics. Inspired by~\cite{Aakerberg2022,BellKligler19,Ji20} we generate $5\times5$-Gaussian kernels $k$ with uniformly random lengths,~\ie~$\sigma_1,\sigma_2\sim\mathcal{U}\left(0.6, 2.5\right)$, and multiplicative noise up to 25\% of the pixels' values,~\ie~$k := k * (1 + 25\%\epsilon), \text{ where }\epsilon\sim\mathcal{N}(0,1)$, to deviate from a regular Gaussian, before normalizing to the sum of 1. The simulated LR images are generated via the well-known model,
\begin{equation}
\label{eq:degradation}
   L = \left(H * k\right)\downarrow_c + n,
\end{equation}
\noindent where $n\sim\mathcal{N}(0, 4)$ models the sensor noise. The kernel and noise distribution are kept hidden from the training process. As aforementioned, for the PMTL scenario, the generated ``true'' LR images are used as training inputs for both tasks, while, in the BSR scenario, \textit{only} for semantic segmentation.

The Vaihingen subset simulates the LR images of interest for super-resolution, whose HR ground truths are not available during training but only semantic annotations. For Potsdam, on the other hand, there exist HR images whose natural LR counterparts are withheld in the BSR setting.
Therefore, the Potsdam subset is used to train super-resolution and Vaihingen for training semantic segmentation as well as testing.
We apply Eq.7 with $c=4$ to the $512\times512$ chips of Vaihingen whose original ground sampling distance (GSD) is 9cm, resulting in LR-HR pairs of resolution $128\times128$ and $512\times512$ with GSD of approximately 36cm and 9cm, respectively.
Conversely, the $512\times512$ chips of Potsdam originally captured at a GSD of 5cm are first downsampled 2 times using the bicubic kernel to clean up possible noises~\cite{Aakerberg2022}, resulting in $256\times256$ HR images with a GSD of 10cm.













\cnes{
\textbf{The Pleiades (CNES/Airbus) dataset\footnote{[Online] Pléiades, Very High-Resolution (50cm) Satellites Imagery \url{https://intelligence.airbus.com/imagery/our-optical-and-radar-satellite-imagery/pleiades/}, accessed November 2024.}} including 230 pan-sharpened images with a GSD at 50cm and a resolution of $2048\times2048\times4$ (R, G, B, and Near-IR) is used as the super-resolution target. The images are treated as LR input for 2-time super-resolution and for training the semantic segmentation task with 9 urban land-cover categories. %
For training the super-resolution branch, a synthetic dataset with representative characteristics of the Pleiades sensor, such as spectral bands, FTM, SNR, is used, which comprises 95 pairs of LR and HR pan-sharpened images with the GSDs of 50cm and 25cm and the dimensions of $812\times812\times4$ and $1624\times1624\times4$, respectively. A sample of each subset is shown in Figure~\ref{fig:CNES_visual_SM}
}


\begin{figure}
    \centering
    \includegraphics[width=0.49\linewidth]{Images/samples/LR4/top_potsdam_2_10_RGBIR-012.png}
    \includegraphics[width=0.49\linewidth]{Images/samples/top_potsdam_2_10_RGBIR-012.png}
    \includegraphics[width=0.49\linewidth]{Images/samples/top_mosaic_09cm_area1-003.png}
    \includegraphics[width=0.49\linewidth]{Images/samples/SS/top_mosaic_09cm_area1-003.png}
    \caption{A sample from the ISPRS dataset with Potsdam $(L_R,H_R)$ (top) and Vaihingen $(L_S, M_S)$ (bottom)
    }
    \label{fig:ISPRS_visual_SM}
\end{figure}

\begin{figure}
    \centering
    \includegraphics[width=0.49\linewidth]{Images/samples/PHR_amiens_10_3_11_reg_simuPELICAN_07.png}
    \includegraphics[width=0.49\linewidth]{Images/samples/PHR_amiens_10_3_11_reg_simuPELICANz_07.png}
    \includegraphics[width=0.49\linewidth]{Images/samples/TOULOUSE_20130924_16bits_COG_9-015-1-4.png}
    \includegraphics[width=0.49\linewidth]{Images/samples/TOULOUSE_9_mask_015-1-4.png}
    \caption{A sample from the simulated dataset (top, $(L_R, H_R)$) and Pléiades images (bottom, $(L_S, M_S)$). The simulated pairs of images follow the statistics of CNES imagery.
    }
    \label{fig:CNES_visual_SM}
\end{figure}

\section{Qualitative Results}

More qualitative results for the blind super-resolution setting are shown in Figure~\ref{fig:qualitatives-blind1_SM} and Figure~\ref{fig:qualitatives-blind2_SM}. State-of-the-art approaches based on natural images' heuristics, such as noise and degradation kernels to augment the inputs, result in blurry or high-frequency artifacts. Although our approach is based on bicubic inputs, using the self-supervised model N2V results in more balanced results of noise and sharpness.

\begin{figure}
    \centering
     \begin{tikzpicture}
        \scriptsize
        \node at (0, 0) {
            \includegraphics[width=\linewidth]{Images/qualitatives-Blinds/top_mosaic_09cm_area13-016_200000.png}
        };
        \node at (-3.0,2.5) {Input (LR)};
        \node at (-1.0,2.5) {Real-SR (STL)};    
        \node at ( 1.0,2.5) {Real-ESR (STL)};
        \node at ( 3.0,2.5) {Bicubic (shared)}; 
        \node at (-3.0,0.0) {Target (4x)};  %
        \node at (-1.0,0.0) {USR-DA (STL)};     
        \node at ( 1.0,0.0) {Real-ESR (hybrid)};
        \node at ( 3.0,0.0) {N2V (hybrid)}; %
    \end{tikzpicture}
    \scriptsize (a)
    \begin{tikzpicture}
        \scriptsize
        \node at (0, 0) {
            \includegraphics[width=\linewidth]{Images/qualitatives-Blinds/top_mosaic_09cm_area7-008_200000.png}
        };
        \node at (-3.0,2.5) {Input (LR)}; 
        \node at (-1.0,2.5) {Real-SR (STL)};
        \node at ( 1.0,2.5) {Real-ESR (STL)};
        \node at ( 3.0,2.5) {Bicubic (shared)};
        \node at (-3.0,0.0) {Target (4x)};  
        \node at (-1.0,0.0) {USR-DA (STL)}; 
        \node at ( 1.0,0.0) {Real-ESR (hybrid)};
        \node at ( 3.0,0.0) {N2V (hybrid)};
    \end{tikzpicture}
    (b)
    \begin{tikzpicture}
        \scriptsize
        \node at (0, 0) {
            \includegraphics[width=\linewidth]{Images/qualitatives-Blinds/top_mosaic_09cm_area21-003_200000.png}
        };
        \node at (-3.0,2.5) {Input (LR)}; 
        \node at (-1.0,2.5) {Real-SR (STL)};
        \node at ( 1.0,2.5) {Real-ESR (STL)};
        \node at ( 3.0,2.5) {Bicubic (shared)};
        \node at (-3.0,0.0) {Target (4x)};  
        \node at (-1.0,0.0) {USR-DA (STL)}; 
        \node at ( 1.0,0.0) {Real-ESR (hybrid)};
        \node at ( 3.0,0.0) {N2V (hybrid)};
    \end{tikzpicture}
    (c)
    \begin{tikzpicture}
        \scriptsize
        \node at (0, 0) {
            \includegraphics[width=\linewidth]{Images/qualitatives-Blinds/top_mosaic_09cm_area21-013_200000.png}
        };
        \node at (-3.0,2.5) {Input (LR)}; 
        \node at (-1.0,2.5) {Real-SR (STL)};
        \node at ( 1.0,2.5) {Real-ESR (STL)};
        \node at ( 3.0,2.5) {Bicubic (shared)};
        \node at (-3.0,0.0) {Target (4x)};  
        \node at (-1.0,0.0) {USR-DA (STL)}; 
        \node at ( 1.0,0.0) {Real-ESR (hybrid)};
        \node at ( 3.0,0.0) {N2V (hybrid)};
    \end{tikzpicture}
    (d)
    \caption{
    Performance of blind super-resolution on ISPRS. Real-SR and Real-ESR-based methods over-smooth the results due to incorrect degradation heuristics, while UDA-SR generates crisp images but with high-frequency artifacts. Naïve bicubic amplifies the input noises, which lessen in the N2V-based results.
    (Best viewed in color and with zoom.)
    }
    \vspace{-2em}
    \label{fig:qualitatives-blind1_SM}
\end{figure}

\begin{figure}
    \centering
     \begin{tikzpicture}
        \scriptsize
        \node at (0, 0) {
            \includegraphics[width=\linewidth]{Images/qualitatives-Blinds/top_mosaic_09cm_area13-002_200000.png}
        };
        \node at (-3.0,2.5) {Input (LR)};
        \node at (-1.0,2.5) {Real-SR (STL)};    
        \node at ( 1.0,2.5) {Real-ESR (STL)};
        \node at ( 3.0,2.5) {Bicubic (shared)}; 
        \node at (-3.0,0.0) {Target (4x)};  %
        \node at (-1.0,0.0) {USR-DA (STL)};     
        \node at ( 1.0,0.0) {Real-ESR (hybrid)};
        \node at ( 3.0,0.0) {N2V (hybrid)}; %
    \end{tikzpicture}
    \scriptsize (a)
    \begin{tikzpicture}
        \scriptsize
        \node at (0, 0) {
            \includegraphics[width=\linewidth]{Images/qualitatives-Blinds/top_mosaic_09cm_area7-010_200000.png}
        };
        \node at (-3.0,2.5) {Input (LR)}; 
        \node at (-1.0,2.5) {Real-SR (STL)};
        \node at ( 1.0,2.5) {Real-ESR (STL)};
        \node at ( 3.0,2.5) {Bicubic (shared)};
        \node at (-3.0,0.0) {Target (4x)};  
        \node at (-1.0,0.0) {USR-DA (STL)}; 
        \node at ( 1.0,0.0) {Real-ESR (hybrid)};
        \node at ( 3.0,0.0) {N2V (hybrid)};
    \end{tikzpicture}
    (b)
    \begin{tikzpicture}
        \scriptsize
        \node at (0, 0) {
            \includegraphics[width=\linewidth]{Images/qualitatives-Blinds/top_mosaic_09cm_area21-015_200000.png}
        };
        \node at (-3.0,2.5) {Input (LR)}; 
        \node at (-1.0,2.5) {Real-SR (STL)};
        \node at ( 1.0,2.5) {Real-ESR (STL)};
        \node at ( 3.0,2.5) {Bicubic (shared)};
        \node at (-3.0,0.0) {Target (4x)};  
        \node at (-1.0,0.0) {USR-DA (STL)}; 
        \node at ( 1.0,0.0) {Real-ESR (hybrid)};
        \node at ( 3.0,0.0) {N2V (hybrid)};
    \end{tikzpicture}
    (c)
    \begin{tikzpicture}
        \scriptsize
        \node at (0, 0) {
            \includegraphics[width=\linewidth]{Images/qualitatives-Blinds/top_mosaic_09cm_area7-012_200000.png}
        };
        \node at (-3.0,2.5) {Input (LR)}; 
        \node at (-1.0,2.5) {Real-SR (STL)};
        \node at ( 1.0,2.5) {Real-ESR (STL)};
        \node at ( 3.0,2.5) {Bicubic (shared)};
        \node at (-3.0,0.0) {Target (4x)};  
        \node at (-1.0,0.0) {USR-DA (STL)}; 
        \node at ( 1.0,0.0) {Real-ESR (hybrid)};
        \node at ( 3.0,0.0) {N2V (hybrid)};
    \end{tikzpicture}
    (d)
    \caption{
    Performance of blind super-resolution on ISPRS. Real-SR and Real-ESR-based methods over-smooth the results due to incorrect degradation heuristics, while UDA-SR generates crisp images but with high-frequency artifacts. Naïve bicubic amplifies the input noises, which lessen in the N2V-based results.
    (Best viewed in color and with zoom.)
    }
    \vspace{-2em}
    \label{fig:qualitatives-blind2_SM}
\end{figure}
